# Supplementary material for: Strange superconductivity near an antiferromagnetic heavy fermion quantum critical point
Source: arXiv:1806.04060 source file (2018-06-11)
Supplement: Supplementary file 1 [file Strange-CeCoIn5-2018-Supp-arXiv.pdf]

# Supplemental Materials of Strange superconductivity near an antiferromagnetic heavy fermion quantum critical point

Y. Y. Chang,[1,*] F. Hsu,[2] S. Kirchner,[3] C. Y. Mou,[2,4] T. K. Lee,[5] and C. H. Chung[1,4,5,†]

[1] *Department of Electrophysics, National Chiao-Tung University, Hsinchu, 300 Taiwan, R.O.C.*
[2] *Department of Physics, National Tsing-Hua University, Hsinchu, 300 Taiwan, R.O.C.*
[3] *Zhejiang Institute of Modern Physics, Department of Physics, Zhejiang University, Hangzhou, P.R.C.*
[4] *Physics Division, National Center for Theoretical Sciences, Hsinchu, 300 Taiwan, R.O.C.*
[5] *Institute of Physics, Academia Sinica, Nankang, Taipei, Taiwan, R.O.C.*

(Dated: June 11, 2018)

In this Supplemental Materials, we provide details of the main text "Strange superconductivity near an antiferromagnetic heavy fermion quantum critical point".

### A: Mean-field results

In this section, we provide details on the mean-field calculations.

The energy dispersion of the itinerant $c$-electrons on a two-dimensional square lattice in the tight-binding formalism reads: $t_{\mathbf{k}} \equiv -2t\,(\cos(k_x a) + \cos(k_y a)) - \mu$ with homogeneous hopping strength $t$. Here, $\mu$ denotes the chemical potential. The lattice constant $a$ is chosen to be a unit of length $a = 1$ throughout the mean-field analysis. While including the Kondo term, $\sum_{\mathbf{k}\sigma=\uparrow\downarrow}(\chi_{\mathbf{k}} c^\dagger_{\mathbf{k}\sigma} f_{\mathbf{k}\sigma} + \text{H.c.})$ (see the main text), the mean-field Hamiltonian reads

$$\begin{aligned} H_{MF} &= \Sigma_{\mathbf{k}\sigma}\, \varphi^\dagger_{\mathbf{k}\sigma} \mathcal{M}_{\mathbf{k}} \varphi_{\mathbf{k}\sigma} \\ &= \Sigma_{\mathbf{k}\sigma} \left( \xi^\alpha_{\mathbf{k}} \alpha^\dagger_{\mathbf{k}\sigma} \alpha_{\mathbf{k}\sigma} + \xi^\beta_{\mathbf{k}} \beta^\dagger_{\mathbf{k}\sigma} \beta_{\mathbf{k}\sigma} \right) \ , \end{aligned} \tag{A.1}$$

where $\varphi_{\mathbf{k}\sigma} \equiv (c_{\mathbf{k}\sigma}, f_{\mathbf{k}\sigma})$, $\lambda$ is the Lagrange multiplier for the local constraint of the $f$-electrons, and the matrix $\mathcal{M}_{\mathbf{k}}$ is given by

$$\mathcal{M}_{\mathbf{k}} \equiv \begin{pmatrix} t_{\mathbf{k}} & \chi_{\mathbf{k}} \\ \chi^*_{\mathbf{k}} & \lambda \end{pmatrix}. \tag{A.2}$$

Here, $\alpha_{\mathbf{k}\sigma}$ ($\beta_{\mathbf{k}\sigma}$) annihilates an electron with spin $\sigma$ and quasi-momentum $\mathbf{k}$ of the bonding (anti-bonding) hybridized bands with the mean-field dispersion relations

$$\begin{aligned} \xi^\alpha_{\mathbf{k}} &= \frac{1}{2}\left[ (t_{\mathbf{k}} + \lambda) - \sqrt{(t_{\mathbf{k}} - \lambda)^2 + 4|\chi_{\mathbf{k}}|^2} \right] \ , \\ \xi^\beta_{\mathbf{k}} &= \frac{1}{2}\left[ (t_{\mathbf{k}} + \lambda) + \sqrt{(t_{\mathbf{k}} - \lambda)^2 + 4|\chi_{\mathbf{k}}|^2} \right] \ . \end{aligned} \tag{A.3}$$

The key point for further mean-field analysis relies on the property that the $\alpha$-band is dominated by the local $f$-electrons since compelling experimental evidences show that heavy-fermion superconductivity is mainly mediated by the local $f$-electrons [1]. For this reason, we only retain the terms involving $\alpha_{\mathbf{k}\sigma}$ in $H_{MF}$ of Eq. (A.1) and neglect the terms containing $\beta_{\mathbf{k}\sigma}$.

The Kondo-induced $d_{x^2-y^2}$-wave superconducting pairing in the hybridized-band basis takes the form $\Delta^\alpha_d(\mathbf{k}) = \Delta_d \cdot (\cos k_x - \cos k_y) \cos^2 \frac{\psi_{\mathbf{k}}}{2}$, with the pair amplitude $\Delta_d = J_H \sum_{\mathbf{k}} (\cos k_x - \cos k_y) \langle f_{\mathbf{k}\uparrow} f_{-\mathbf{k}\downarrow} \rangle$. Finally, the resulting Bogoliubov quasi-particle dispersion is then given by $E^\alpha_{\mathbf{k}} = \sqrt{{\xi^\alpha_{\mathbf{k}}}^2 + \Delta^\alpha_d(\mathbf{k})^2}$ .

Various temperature-dependent mean-field variables such as the Kondo hybridization $\chi$, the RVB pairing amplitude $\Delta$ and the Lagrange multiplier $\lambda$ in the mean-field Kondo-Heisenberg model are solved self-consistently from

$$\begin{aligned} &\frac{J_H}{N_s} \sum_{\mathbf{k}} \frac{\phi^2_{\mathbf{k}}}{2E^\alpha_{\mathbf{k}}} \tanh \frac{E^\alpha_{\mathbf{k}}}{2k_B T} = 1 \ , \quad \chi_{\mathbf{k}} = J_K \sum_\sigma \langle c^\dagger_{\mathbf{k}\sigma} f_{\mathbf{k}\sigma} \rangle \ , \\ &n_f(\lambda) = \frac{1}{N_s} \sum_{\mathbf{k}\sigma} \langle f^\dagger_{\mathbf{k}\sigma} f_{\mathbf{k}\sigma} \rangle \ , \end{aligned} \tag{A.4}$$

where

$$\begin{aligned} \phi_{\mathbf{k}} &= (\cos k_x - \cos k_y) \cos^2 \frac{\psi_{\mathbf{k}}}{2} \ , \\ \cos^2 \frac{\psi_{\mathbf{k}}}{2} &= \frac{1}{2}\left[ 1 + \frac{(t_{\mathbf{k}} - \lambda)/2}{\sqrt{\left(\frac{t_{\mathbf{k}}-\lambda}{2}\right)^2 + |\chi|^2}} \right] \ . \end{aligned} \tag{A.5}$$

Note that the valence fluctuation of the local $f$-electrons is considered in our mean-field analysis in Eq. (A.4), i.e. $n_f < 1$, as suggested by the x-ray absorption experiments (experimentally $0.8 < n_f < 0.9$) [3,4].

The specific heat coefficient is obtained via [5]

$$\frac{C_V}{N_s} = 2k_B \sum_{\mathbf{k}} \frac{e^{\beta E^\alpha_{\mathbf{k}}}}{(1 + e^{\beta E^\alpha_{\mathbf{k}}})^2} \cdot \left( \frac{E^{\alpha 2}_{\mathbf{k}}}{k_B^2 T^2} - \frac{1}{2k_B^2 T} \frac{d{E^\alpha_{\mathbf{k}}}^2}{dT} \right) \ . \tag{A.6}$$

We find, by choosing $J_K/t = 1.2$, $J_H/t = 1.0$, $n_f = 0.8$ and $\mu/t = -0.12$ with $t \sim 300$K (a reasonable estimation from the ARPES measurement [6]), that all the characteristic temperature scales including the onset temperature of Kondo hybridization $T^*_{\text{onset}}$, the coherent temperature $T^*_{coh}$ and superconducting transition temperature $T_c$ as well as the specific heat coefficient $\gamma(T)$ in the superconducting regime can be well accounted for. The mean-field analysis (see Fig. A.1) gives $T^*_{\text{onset}} \sim 90$K, $T^*_{coh} = \chi^2(T = 0)/D$ [4] ($D \sim 2t$ is the estimated half bandwidth of the $f$-electron-dominated hybridized band $\xi^\alpha_{\mathbf{k}}$ in Eq. (A.3)), $T_c \sim 0.007t \sim 2$K. The relations

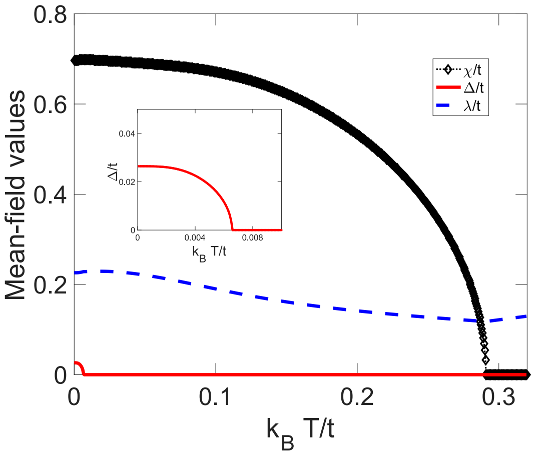


FIG. A.1: The plot of the time-dependent mean-field variables: We choose $J_K/t = 1.2$, $J_H/t = 1.0$ and the chemical potential $\mu/t = -0.12$ in unit of the hopping strength $t$. In this plot, we choose the occupation number per site of the local $f$-electrons $n_f$ to be 0.8 due to the valence fluctuation. The inset shows the enlarged plot of $\Delta/t$.

$T_c \ll T^*_{coh} \ll T^*_{\text{onset}}$ and the ratio $T^*_{coh}/T_c \sim 30$ are both consistent with that observed in experiments [7,8]. The result of the specific heat coefficient in the superconducting regime, obtained via Eq. (A.6), is shown in Fig. 1(c) of the main text.

We further find that the onset temperature of Kondo hybridization $T^*_{\text{onset}}$ versus the Kondo coupling $J_K$ follows a similar relation to the single-impurity Kondo scale

$$k_B T^*_{\text{onset}} = D \exp(-1/J_K \rho_0) \tag{A.7}$$

with $\rho_0$ being the density of state at Fermi level. The result is illustrated in Fig. A.2.

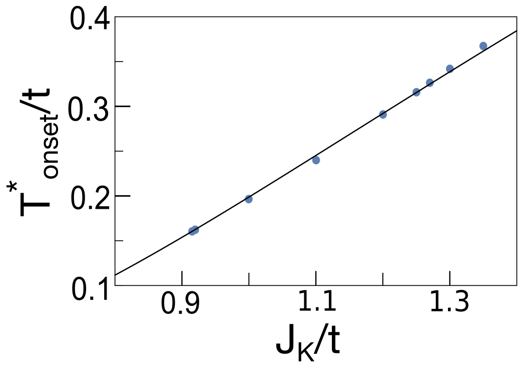


FIG. A.2: The onset temperature $T^*_{\text{onset}}$ versus the Kondo coupling $J_K$: $T^*_{\text{onset}}$ is determined from the mean-field calculation (blue dots). We fit the data to the single-impurity Kondo scale in Ref. 9 (the solid line).

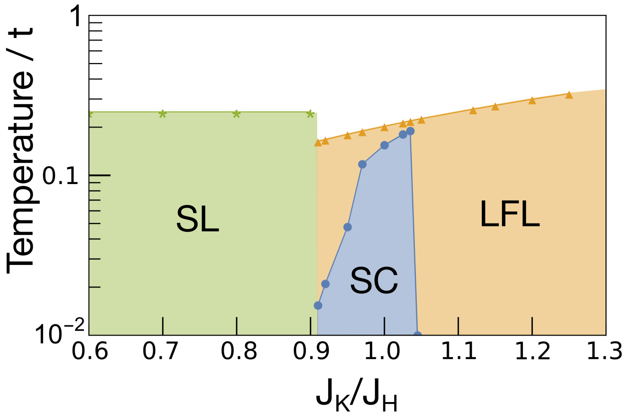


FIG. A.3: The mean-field phase diagram with $B \sim 5$T and $n_f \sim 0.95$ for a nearly half-filled local $f$-band.

### 1. Mean field results at a finite magnetic field

To support the RG calculation near the borderline of the AF, superconducting and Kondo (LFL) phases, we include the magnetic field as a Zeeman term $H_B$ in the mean-field Hamiltonian.

Without loss of generality, we assume the magnetic field is along the $z$-direction. The Zeeman term $H_B$ thus takes the form

$$H_B = -\sum_{i,\sigma=\pm} \sigma \left( h_c c^\dagger_{i,\sigma} c_{i,\sigma} + h_f f^\dagger_{i,\sigma} f_{i,\sigma} \right) \tag{A.8}$$

with $h_c = e\hbar B/2m^*_c$ and $h_f = e\hbar B/2m^*_f$ being Zeeman splitting energy for the $c$- and $f$-electron, respectively. The effective mass of the mobile $c$ electrons $m^*_c$ and the localized $f$-electrons $m^*_f$ are determined from Ref. 6, which gives $m^*_c \sim m_e$ and $m^*_f \sim 20\, m_e$ ($m_e$ being the free electron mass) from the ARPES measurements. The Zeeman splitting energy $h_c$ of the $c$-electrons can be easily evaluated through $h_c = \mu_B B$ with $\mu_B \equiv e\hbar/2m_e \approx 6\times10^{-5}$ eV/T being the Bohr magneton of free electrons.

In the presence of magnetic field and doping ($B \sim 5$T, corresponding to $h_c/t \approx 10^{-2}$, and $n_f \sim 0.95$), we find that the range of the superconducting dome significantly shrinks, as shown in Fig. A.3, consistent with experiments [2].

## B: Dispersions for the boson fields

The dispersion relations for the bosonic Gaussian fields of amplitude fluctuation, $\hat{\tilde{\chi}}$ and $\hat{\tilde{\Phi}}$, are obtained via integrating out the high-energy modes on the Fermi surface of the conduction $c$-electrons. First, we compute the self-energy corrections, $\Sigma_\chi$ and $\Sigma_\Phi$, up to the first order of $\hat{\tilde{\chi}}$ and $\hat{\tilde{\Phi}}$, respectively, and modified their bare Green's function via $\Sigma_\chi$ and $\Sigma_\Phi$ through Dyson equation:

$$G^{-1}_{\chi,\Phi} = \left(G^b_{\chi,\Phi}\right)^{-1} - \Sigma_{\chi,\Phi}. \tag{B.1}$$

The following derivations are outlined from Ref. 10.

### 1. Dispersion for $\hat{\tilde{\chi}}$

We first compute $\Sigma_\chi$. Since the $\hat{\tilde{\chi}}_i$ field is a real boson in the real space, thus, the Fourier component of $\hat{\tilde{\chi}}_i$ follows $\hat{\tilde{\chi}}_{\mathbf{k}} = \hat{\tilde{\chi}}^\dagger_{-\mathbf{k}}$, similar in form to a phonon operator. Thus, $\hat{\tilde{\chi}}_{\mathbf{k}}$ can be written as

$$\hat{\tilde{\chi}}(\mathbf{k}) = b_\chi(\mathbf{k}) + b^\dagger_\chi(-\mathbf{k}), \tag{B.2}$$

leading the following form for the Kondo term:

$$J_\chi \sum_{\mathbf{k},\mathbf{k}',\sigma} \left[ c^\dagger_{\mathbf{k},\sigma} f_{\mathbf{k}',\sigma} \left( b^\dagger_\chi(\mathbf{k}'-\mathbf{k}) + b_\chi(-\mathbf{k}'+\mathbf{k}) \right) + \text{H.c.} \right] + \frac{2|b_\chi(\mathbf{k})|^2}{J_\chi}. \tag{B.3}$$

In terms of the $b$ bosons, the Green's function $G_\chi$ can be rewritten as

$$\begin{aligned} &G_\chi(\mathbf{k},\tau) \\ =& -\langle T_\tau b_\chi(\mathbf{k},\tau) b^\dagger_\chi(\mathbf{k},0)\rangle - \langle T_\tau b^\dagger_\chi(-\mathbf{k},\tau) b_\chi(-\mathbf{k},0)\rangle \\ \equiv& G_{b_\chi}(\mathbf{k},\omega) + G_{\bar{b}_\chi}(\mathbf{k},\omega), \end{aligned} \tag{B.4}$$

where we define $\bar{b}_\chi(\mathbf{k}) \equiv b^\dagger_\chi(-\mathbf{k})$. In Eq. (B.4), we do not consider the off-diagonal part of $G_\chi$ since we are only interested in the parameter regime near the QCP where the Kondo fluctuation is not Bose-condensed. The dispersion of $\hat{\tilde{\chi}}$ can be extracted from the Dyson equations:

$$G^{-1}_{b_\chi} = -1/J_\chi - \Sigma_{b_\chi},\ G^{-1}_{\bar{b}_\chi} = -1/J_\chi - \Sigma^*_{b_\chi}. \tag{B.5}$$

The above arguments can be directly applied to the $\hat{\tilde{\Phi}}$ boson, see the next subsection for details.

Up to the one-loop order, we have

$$\begin{aligned} &\Sigma_{b_\chi}(\mathbf{k},\omega) \\ =& \left( N_0 J_\chi^2 \left( \int_{\Lambda-\varepsilon_c(\mathbf{k})}^{\Lambda} + \int_{-\Lambda}^{-\Lambda+\varepsilon_c(\mathbf{k})} \right) \frac{n_f(\varepsilon')\, d\varepsilon'}{i\omega + \varepsilon' - \lambda} \right) \\ \approx& N_0 J_\chi^2 \ln \left[ \frac{i\omega - \Lambda - \lambda + \varepsilon_c(\mathbf{k})}{-\lambda} \right] \\ \approx& \frac{N_0 J_\chi^2}{\lambda} \left( -i\omega - \frac{k^2}{2m^*} + \Lambda \right). \end{aligned} \tag{B.6}$$

The self-energy correction up to second order in $J_\chi$ generates a quadratic dispersion for the $\hat{\tilde{\chi}}$ boson due to the quadratic dispersion for the $c$ electrons: $\varepsilon_c(\mathbf{k}) = k^2/2m^*$.

Similarly, the self-energy correction for $\bar{b}_\chi(\mathbf{k})$ is given by

$$\Sigma_{\bar{b}_\chi}(\mathbf{k},\omega) = \Sigma^*_{b_\chi}(\mathbf{k},\omega) = \frac{N_0 J_\chi^2}{\lambda} \left( i\omega - \frac{k^2}{2m^*} + \Lambda \right). \tag{B.7}$$

Adding up $G_{b_\chi}$ and $G_{\bar{b}_\chi}$, we find

$$\begin{aligned} G_\chi(i\omega,\mathbf{k}) =& \frac{1}{i\omega_\chi + \frac{N_0 J_\chi^{*\,2} k^2}{2m^*\lambda} - \frac{N_0 J_\chi^{*\,2}\Lambda}{\lambda} - 1/J^*_\chi} \\ &- \frac{1}{i\omega_\chi - \frac{N_0 J_\chi^{*\,2} k^2}{2m^*\lambda} + \frac{N_0 J_\chi^{*\,2}\Lambda}{\lambda} + 1/J^*_\chi}, \end{aligned} \tag{B.8}$$

where, in Eq. (B.8), we define $\omega_\chi \equiv \frac{N_0 J_\chi^{*\,2}\omega}{\lambda}$ with $J_\chi$ being fixed at its fixed-point value $J^*_\chi$. The Taylor expansion of $\ln(1+x) \approx x$ has also been used in Eq. (B.8). The mass for the $\hat{\tilde{\chi}}$ boson is found to be $m_\chi = \frac{N_0 J_\chi^{*\,2}\Lambda}{\lambda} + 1/J^*_\chi \approx 1/J^*_\chi$.

### 2. Dispersion for $\hat{\tilde{\Phi}}$

Now, we turn to the calculation of the self-energy correction for the $\hat{\tilde{\Phi}}$ field.

Similar to the previous calculations for the dispersion of the $\hat{\tilde{\chi}}$ field, we rewrite the amplitude-fluctuating RVB operators as $\hat{\tilde{\Phi}}(\mathbf{k}) = b_\Phi(\mathbf{k}) + \bar{b}_\Phi(\mathbf{k})$ with $\bar{b}_\Phi(\mathbf{k}) \equiv b^\dagger_\Phi(-\mathbf{k})$, the Green's function $G_\Phi$ can be expressed as a summation of the Green's functions $G_{b_\Phi}$ and $G_{\bar{b}_\Phi}$ for the $b_\Phi(\mathbf{k})$ and $\bar{b}_\Phi(\mathbf{k})$ operators, respectively. While expressing the RKKY interaction $S_J$ in terms of $b_\Phi(\mathbf{k})$ and $\bar{b}_\Phi(\mathbf{k})$, the bare Green's functions for $b_\Phi$ and $\bar{b}_\Phi$ can be shown to identical to each other: $G^b_{b_\Phi} = G^b_{\bar{b}_\Phi} = -(1/J_\Phi)^{-1}$.

The lowest non-trivial contribution is found to be from the fourth-order perturbation in $J_\Phi^2 J_\chi^2$, see the corresponding Feynman diagram in Fig. B.1(the second-order self-energy correction in $J_\Phi$ (see Fig. C.3(d)) does not contribute any momentum-dependent corrections to the dispersion of the $\hat{\tilde{\Phi}}$ bosons), given by

$$\Sigma_\Phi(\omega) = -\frac{2J_\Phi^2}{\lambda + \Sigma_f^{(2)}(\omega)}, \tag{B.9}$$

where

$$\Sigma_f^{(2)}(\mathbf{k},\omega) \approx \frac{4N_0 J_\chi^2\, i\omega}{\Lambda} + \frac{N_0 J_\chi^2}{m^*\Lambda} k^2. \tag{B.10}$$

Thus, the self-energy correction to the Green's function $G_{b_\Phi}$ can be evaluated as

$$\begin{aligned} \Sigma^{(2)}_{b_\Phi}(\mathbf{k},\omega) =& -\frac{2J_\Phi^2}{\lambda} \left( \frac{1}{1 + \frac{4N_0 J_\chi^2\, i\omega}{\Lambda\lambda} + \frac{N_0\, J_\chi^2}{m^*\,\lambda(\Lambda+\omega)} k^2} \right) \\ \approx& -\frac{2J_\Phi^2}{\lambda} + i\omega_\Phi + \frac{2N_0 J_\chi^2 J_\Phi^2}{m^*\,\lambda^2\,\Lambda} k^2, \end{aligned} \tag{B.11}$$

and the modified Green's function $G_{b_\Phi}$ including the self-energy correction is thus given by

$$G^{-1}_{b_\Phi} \approx -\frac{1}{J_\Phi} - i\omega_\Phi - \frac{2N_0 J_\chi^2 J_\Phi^2}{m^*\,\lambda^2\,\Lambda} k^2, \tag{B.12}$$

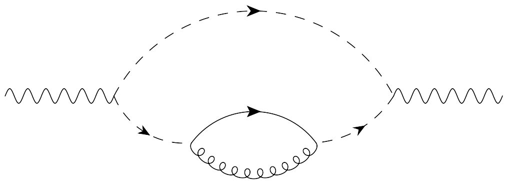

FIG. B.1: The self energy diagram in RPA contributed to the dispersion of $\hat{\tilde{\Phi}}_k$ field. Various propagators shown in this figure are defined in Fig. C.1.

where we define $\omega_\Phi \equiv \frac{8N_0 J_\chi^{*\,2} J_\Phi^{*\,2}\,\omega}{\Lambda\lambda^2}$ with all the couplings being fixed at its fixed point values. The Green's function for $\hat{\tilde{\Phi}}$ thus reads

$$G_\Phi^b(i\omega,\,\mathbf{k}) \approx \frac{1}{-\frac{1}{J_\Phi^*} - i\omega_\Phi - \frac{2N_0 J_\chi^{*\,2} J_\Phi^{*\,2}}{m^*\,\lambda^2\,\Lambda}\,k^2} + \frac{1}{-\frac{1}{J_\Phi^*} + i\omega_\Phi - \frac{2N_0 J_\chi^{*\,2} J_\Phi^{*\,2}}{m^*\,\lambda^2\,\Lambda}\,k^2}. \quad \text{(B.13)}$$

According to the Dyson's equation, the dispersion for $\hat{\tilde{\Phi}}$ is given by $\varepsilon_\Phi(\mathbf{k}) = \frac{2N_0 J_\chi^{*\,2} J_\Phi^{*\,2}}{m^*\,\lambda^2\,\Lambda^2}\,k^2$ and the bare mass for the $\hat{\tilde{\Phi}}$ boson is defined as $m_\Phi = 1/J_\Phi^*$.

## C: RG analysis

In this section, we apply the perturbative renormalization group (RG) approach in the weak coupling regime to study the competition between various interactions of the effective action in Eq. (1) of the main text near the QCPs $g_{c1}$ (in Section C 1) and $g_{c2}$ (in Section C 2), respectively. We also derive the RG equations shown in Eqs. (2) and (3) of the main text. The RG procedures primarily include determining the bare scaling dimension of various fields (operators) and coupling constants, the derivations for the self-energy and vertex corrections.

The wave vector $k$, Fermi momentum $k_F$ and the frequency $\omega$ are rescaled as

$$k' = e^l k\ ,\ \ k_F' = e^l k_F\ ,\ \ \omega' = e^{zl}\omega\ , \quad \text{(C.1)}$$

where the dynamical exponent $z = 2$. Here, we take a circular Fermi surface of the $c$ electrons to simplify our RG treatment. Experimentally, the ARPES measurement shows that the $\beta$ bands for both $CeCoIn_5$ and $CeRhIn_5$ are almost circular at low temperature [6,20], indicating that a circular Fermi surface in the RG approach is a reasonable assumption. It is worthwhile mentioning that we allow the Fermi momentum $k_F$ to flow in the same way as the quasi-momentum $\mathbf{k}$ in our RG scheme, similar to Refs. 10 and 11. This approach is distinct from the patch RG scheme on a two dimensional Fermi surface [12] at which the Fermi volume is conserved due to the Luttinger theorem. We also assume that the self energy only depends on external frequency but is independent of external momentum. A similar approach can be found in Refs. 10,13,14.

Fig. C.1 shows the diagrammatic representations for various bare propagators:

$$G_c^b(\omega,\mathbf{k}) = \frac{1}{i\omega - \varepsilon_c(\mathbf{k})}\ ,$$
$$G_f^b(\omega,\mathbf{k}) = \frac{i\omega+\lambda}{(i\omega)^2 - E^2(\mathbf{k})} \approx \frac{1}{i\omega-\lambda}\ ,$$
$$G_{\chi,\Phi}^b(\omega,\mathbf{k}) = \frac{2(\varepsilon_{\chi,\Phi}(\mathbf{k}) + m_{\chi,\Phi})}{(i\omega_{\chi,\Phi})^2 - (\varepsilon_{\chi,\Phi}(\mathbf{k}) + m_{\chi,\Phi})^2}\ , \quad \text{(C.2)}$$

where $E(\mathbf{k}) = \sqrt{\lambda^2 + |\Phi(\mathbf{k}) + \Phi(-\mathbf{k})|^2}$ with $\Phi(\mathbf{k}) \equiv 2\Delta_d(\cos k_x - \cos k_y) \approx \sqrt{\lambda^2 + 64|\Delta_d|^2}$ (the definition of $\Delta_d$ is shown in Section A). The Green's functions for the real bosons come from the self-energy corrections, see Section B. Near the QCP, we can approximate $\lambda \to \infty$ at the end of calculation (see Refs. 15 and 16 for detailed explanation), leading to $E(\mathbf{k}) \approx \lambda$. Thus, the Green's function of the $f$-electron can be reduced to the regular (diagonal) part, and the off-diagonal Green's functions are neglected.

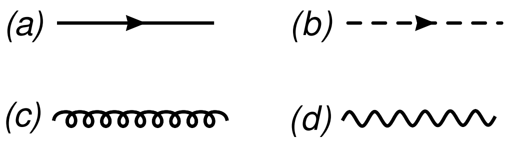


FIG. C.1: The diagrammatic representation of various bare propagators: (a) the conduction electrons (solid line), (b) the local $f$-electrons (dashed line), (c) the fluctuating Kondo correlation $\hat{\tilde{\chi}}$ (helical line) and (d) the fluctuating spin-singlet RVB correlation $\hat{\tilde{\Phi}}$ (wavy line).

### 1. RG near $g_{c1}$: Spin liquid (SL)-to-superconducting (SC) phase transition

The Feynman diagrams for the self energies relevant for the spin liquid-to-superconducting phase transition ($g_{c1}$) are illustrated in Figs. C.2(c) (for the local $f$-electron) and (d) (for the $\hat{\tilde{\chi}}$ field).

The contribution from Fig. C.2(c), denoted as $\Sigma_f^{(2)}$, is given by

$$\Sigma_f^{(2)}(i\omega) = \frac{2J_\chi^2}{\beta}\sum_{i\nu}\sum_{\mathbf{k}} G_c^b(i\nu,\mathbf{k})G_\chi^b(i\omega - i\nu,\mathbf{k})$$
$$= \frac{2J_\chi^2}{\beta}\sum_{i\nu,\,\mathbf{k}} \frac{1}{i\nu - \varepsilon_c(\mathbf{k})}\left[\frac{1}{i\omega - i\nu - \varepsilon_\chi(\mathbf{k}) - m_\chi} - \frac{1}{i\omega - i\nu + \varepsilon_\chi(\mathbf{k}) + m_\chi}\right]. \quad \text{(C.3)}$$

Here, the approximate $\varepsilon_c(\mathbf{k}) \pm \varepsilon_\chi(\mathbf{k}) \approx \varepsilon_c(\mathbf{k})$ is used since $\varepsilon_\chi(\mathbf{k})$ compared with $\varepsilon_c(\mathbf{k})$ is a higher order term, i.e.

$\varepsilon_\chi(\mathbf{k}) \ll \varepsilon_c(\mathbf{k})$. Thus,

$$\begin{aligned} \Sigma_f^{(2)}(i\omega) &= -2J_\chi^2 \sum_{\mathbf{k}} \frac{1}{i\omega - \varepsilon_c(\mathbf{k})} \\ &= -2J_\chi^2 N_0 \int_{-\Lambda}^{\Lambda} \frac{d\varepsilon}{i\omega - \varepsilon} \sim (\ln \Lambda)^0 \ . \end{aligned} \tag{C.4}$$

Fig. C.2(c) gives no logarithmic divergence.

Similarly, the contribution from Fig. C.2(d) is

$$\begin{aligned} \Sigma_\chi(i\omega) &= \frac{2J_\chi^2}{2!\cdot\beta} \sum_{i\nu}\sum_{\mathbf{k}} G_f^b(i\omega + i\nu) G_c^b(i\nu, \mathbf{k}) \\ &= J_\chi^2 \sum_{\mathbf{k}} \frac{1}{i\omega + \varepsilon_c(\mathbf{k}) - \lambda} \ . \end{aligned} \tag{C.5}$$

The result of Fig. C.2(d) reads

$$\begin{aligned} \Sigma_\chi(\omega + \lambda) &= J_\chi^2 N_0 \int_{-\Lambda}^{\Lambda} d\varepsilon \, \frac{n_F(\varepsilon)}{\omega + \varepsilon} \\ &\approx -J_\chi^2 N_0 \ln \frac{\Lambda}{\omega} \ . \end{aligned} \tag{C.6}$$

Now, we turn to the vertext corrections for $v_{sc}$. There are two contributions, as shown in Figs. C.2(e) and (f). The vertex correction $\Gamma^{(1)}$ for Fig. C.2(e) is given by

$$\begin{aligned} \Gamma^{(1)}(k_1 + k_2) &= \frac{6}{3!}\frac{v_{sc}^3}{\beta^2} \sum_{\nu_1,\nu_2}\sum_{\mathbf{q}_1,\mathbf{q}_2} G_\chi^b(-k_1 - k_3 - q_1) G_\chi^b(k_1 + k_3 - q_2) G_c^b(q_1) G_c^b(q_2) \\ &= \frac{6}{3!}\frac{v_{sc}^3}{\beta^2} \sum_{\nu_1,\nu_2}\sum_{\mathbf{q}_1,\mathbf{q}_2} \frac{1}{i\nu_1 - \varepsilon_{\mathbf{q}_1}} \cdot \frac{1}{i\nu_2 - \varepsilon_c(\mathbf{q}_2)} \\ &\quad \cdot \left[ \frac{1}{i(\omega_1 + \omega_3 - \nu_2) - \varepsilon_\chi(\mathbf{k}_1 + \mathbf{k}_3 - \mathbf{q}_2)} - \frac{1}{i(\omega_1 + \omega_3 - \nu_2) + \varepsilon_\chi(\mathbf{k}_1 + \mathbf{k}_3 - \mathbf{q}_2)} \right] \\ &\quad \cdot \left[ \frac{1}{i(\omega_1 + \omega_3 - \nu_2) - \varepsilon_\chi(\mathbf{k}_1 + \mathbf{k}_3 - \mathbf{q}_2)} - \frac{1}{i(\omega_1 + \omega_3 - \nu_2) + \varepsilon_\chi(\mathbf{k}_1 + \mathbf{k}_3 - \mathbf{q}_2)} \right] \ , \end{aligned} \tag{C.7}$$

where we have defined $k_i \equiv (\omega_i, \mathbf{k}_i)$ being a vector contains the frequency and momentum for the external legs while $q_i \equiv (\nu_i, \mathbf{q}_i)$ for the internal propagators. To simplify the calculation, we take the approximation $\varepsilon_c \gg \varepsilon_\chi$, leading to

$$\begin{aligned} \Gamma^{(1)}(k) &= \left(-\frac{6\, v_{sc}^3}{3!}\right) \sum_{\mathbf{q}_1,\mathbf{q}_2} \frac{1}{i\omega - \varepsilon_c(\mathbf{q}_1)} \cdot \frac{1}{i\omega + \varepsilon_c(\mathbf{q}_2)} \\ &= -\frac{v_{sc}^3 N_0^2}{\omega} d\ln\Lambda \ , \end{aligned} \tag{C.8}$$

where $k \equiv (\omega, \mathbf{k}) \equiv (\omega_1 + \omega_3, \mathbf{k}_1 + \mathbf{k}_3)$.

The next step is to introduce the field (Green's function) and coupling (vertex) function renormalization [13,14]. After reducing the cutoff $\Lambda$ to $\Lambda'$ ($\Lambda' < \Lambda$), these renormalizations are determined via

$$\gamma_{j_\chi}(\Lambda') = Z_{j_\chi}^{-1}\gamma_{j_\chi}(\Lambda) \ , \ \gamma_{v_{sc}}(\Lambda') = Z_{v_{sc}}^{-1}\gamma_{v_{sc}}(\Lambda) \ , \tag{C.9}$$

and

$$\mathcal{G}_f(\omega,\ \Lambda') = Z_f \mathcal{G}_f(\omega,\ \Lambda) \ , \ \mathcal{G}_\chi(\omega,\ \Lambda') = Z_\chi \mathcal{G}_\chi(\omega,\ \Lambda) \ , \tag{C.10}$$

where the $Z$-factors can be obtained from the diagrammatic calculation above.

The coupling constant renormalization near $g_{c1}$ is therefore defined as:

$$j_\chi = Z_{j_\chi} Z_f^{-\frac{1}{2}} Z_\chi^{-\frac{1}{2}} J_\chi \ , \ v_{sc}^R = Z_{v_{sc}} Z_\chi^{-1} v_{sc}^b \ . \tag{C.11}$$

In Eq. (C.11), the subscript $b$ denotes "bare" while $R$ means "renormalized". With the help of the $Z$'s defined in Eqs. (C.9) and (C.10) above, the RG $\beta$ functions can be obtained as

$$Z_f = 1 \ , \ Z_\chi = 1 + j_\chi^2 \cdot d\ln\Lambda \ , \tag{C.12}$$

and

$$Z_{j_\chi} = 1 \ , \ Z_{v_{sc}} = 1 + 12 v_{sc}^3 \cdot d\ln\Lambda \ . \tag{C.13}$$

The RG equations for $j_\chi$ and $v_{sc}$ are obtained by Eqs. (C.12) and (C.13) as:

$$\begin{aligned} \frac{dj_\chi}{dl} &= \left(-\frac{\epsilon}{2}\right) j_\chi + \frac{1}{2} j_\chi^3 \ , \\ \frac{dv_{sc}}{dl} &= -\epsilon v_{sc} + j_\chi^2 v_{sc} + 12 v_{sc}^3 \end{aligned} \tag{C.14}$$

with $\epsilon \equiv d - z$ and $dl = -\ln d\Lambda$ is defined. Except for the Gaussian fixed point $(j_\chi^{2^*},\ v_{sc}^{2^*}) = (0,\ 0)$, the RG $\beta$ functions in Eq. (C.14) yield two non-trivial fixed points at $(j_\chi^{2^*},\ v_{sc}^{2^*}) = (\epsilon,\ 0)$ and $(j_\chi^{2^*},\ v_{sc}^{2^*}) = (0,\ \epsilon/12)$.

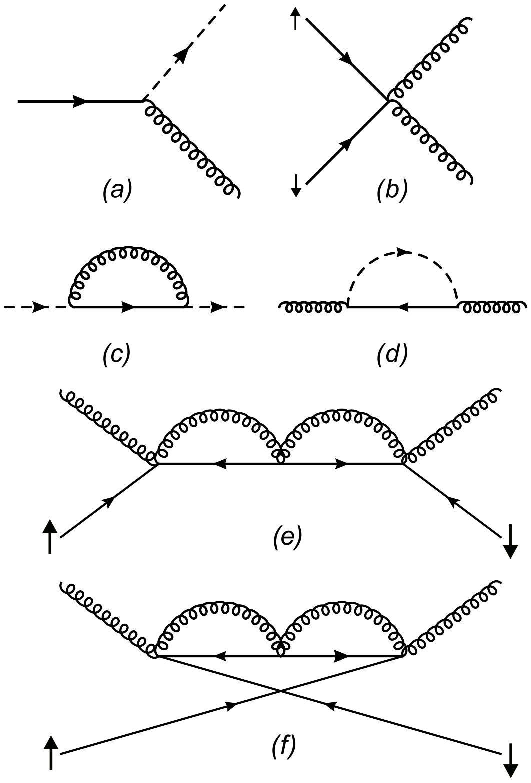


FIG. C.2: The Feynman diagrams relevant for the spin liquid-to-superconducting state transition near $g_{c1}$. The interaction vertices for the Kondo coupling $J_\chi$ and the superconductivity are shown in (a) and (b). The Feynman diagrams for the one-loop self energy for (c) the local $f$-electrons and (d) the $\hat{\tilde{\chi}}$ field. (e) and (f) show the vertex correction to the one-loop order for the $v_{sc}$ coupling.

### 2. RG near $g_{c2}$: Superconducting (SC) phase-to-Kondo (LFL) transition

We now perform the RG analysis near $g_{c2}$. First, we calculate the one-loop correction to the self energy of the RVB spin-singlet fluctuation $\hat{\tilde{\Phi}}_k$ field. The first contribution comes from Fig. C.3(d), given by

$$\Sigma_\Phi^{(1)}(\tau) = -\frac{8}{2!}\cdot J_\Phi^2 G_f^b(\tau) G_f^b(\tau) \ , \tag{C.15}$$

where $0 < \tau < \beta$. The bare Green's function of the $f$-electron, $G_f^b$, as a function of imaginary time $\tau$ is defined as

$$\begin{aligned} G_f^b(\tau) &= e^{-\lambda\tau}\left[(n_F(\lambda)-1)\Theta(\tau) + n_F(\lambda)\Theta(-\tau)\right] \\ &= e^{-\lambda\tau}\left[n_F(\lambda)-1\right] \ , \end{aligned} \tag{C.16}$$

where $\Theta(\tau)$ is the unit-step function and $n_F(y) = \left(e^{\beta y}+1\right)^{-1}$ is the Fermi-Dirac distribution function. After taking $\lambda\to\infty$, $\Sigma_\Phi(\tau)$ vanishes.

Similarly, the other contribution to the self energy of $\hat{\tilde{\Phi}}$ comes from Fig. C.3(e) (denoted as $\Sigma_\Phi^{(2)}$),

$$\begin{aligned} \Sigma_\Phi^{(2)}(i\omega) &= -\frac{2v_{sc}^2}{\beta}\sum_{i\nu,\mathbf{k}} G_c^b(i\omega - i\nu,\mathbf{k}) G_c^b(i\nu,-\mathbf{k}) \\ &= -\frac{2v_{sc}^2}{\beta}\sum_{i\nu,\mathbf{k}} \frac{1}{i\omega - i\nu - \varepsilon_c(\mathbf{k})}\times\frac{1}{i\nu-\varepsilon_c(-\mathbf{k})}. \end{aligned} \tag{C.17}$$

Due to parity symmetry, we have $\varepsilon_c(\mathbf{k}) = \varepsilon_c(-\mathbf{k})$, leading to

$$\begin{aligned} \Sigma_\Phi^{(2)}(i\omega) &= -2v_{sc}^2\sum_{\mathbf{k}}\left[\frac{n_F(\varepsilon_c(\mathbf{k}))}{i\omega - 2\varepsilon_c(\mathbf{k})} - \frac{n_F(i\omega-\varepsilon_c(\mathbf{k}))}{i\omega-2\varepsilon_c(\mathbf{k})}\right] \\ &= -2v_{sc}^2 N_0\int_{-\Lambda}^{\Lambda}\frac{2n_F(\varepsilon)-1}{i\omega-2\varepsilon}d\varepsilon \ . \end{aligned} \tag{C.18}$$

Applying the technique of Cauchy principal value, the result for $\Sigma_\Phi^{(2)}$ reads

$$\Sigma_\Phi^{(2)}(\omega) \approx -2v_{sc}^2 N_0 \ln\frac{\Lambda}{\omega} + \mathcal{O}(\omega) \ . \tag{C.19}$$

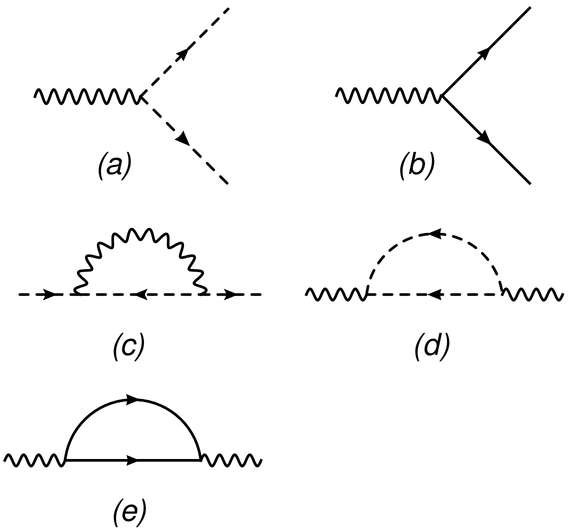


FIG. C.3: The relevant Feynman diagrams for the RG $\beta$ functions for the transition from the coexisting superconducting state to the Kondo state near $g_{c2}$. (a) and (b) show the bare vertex for the $J_\Phi$ and $v_{sc}$ couplings. (c), (d) and (e) illustrate the self energies to the one-loop order.

The self energy correction to the $f$-electron Green's function near $g_{c2}$ only comes from the second order perturbation in $J_\Phi$ (represented by $\Sigma_f^{(1)}$), as specified in Fig.

C.3(c), given by

$$\begin{aligned}\Sigma_f^{(1)}(i\omega) &= \frac{8\cdot J_\Phi^2}{2!\cdot\beta}\sum_{i\nu}\sum_{\mathbf{k}} G_\Phi^b(-i\omega-i\nu,\mathbf{k})G_f^b(i\nu)\\ &= -\frac{4J_\Phi^2}{\beta}\sum_{i\nu}\sum_{\mathbf{k}}\left(\frac{1}{i\omega+i\nu+\epsilon_\Phi(\mathbf{k})}-\frac{1}{i\omega+i\nu-\epsilon_\Phi(\mathbf{k})}\right)\\ &\times\frac{1}{i\nu-\lambda}\\ &= 4J_\Phi^2\sum_{\mathbf{k}}\frac{n_B(\epsilon_\Phi(\mathbf{k}))+1}{i\omega+\epsilon_\Phi(\mathbf{k})+\lambda}\ . \end{aligned}\tag{C.20}$$

$n_B(\epsilon) = (e^{\beta\epsilon}-1)^{-1}$ is the Bose-Einstein distribution. Setting $i\omega=\omega-\lambda$ and $\lambda\to\infty$ at the end of calculation, we have

$$\begin{aligned}\Sigma_f^{(1)}(\omega-\lambda) &= 4J_\Phi^2K_0\int_0^\Lambda\frac{d\epsilon}{\omega+\epsilon}\\ &\approx 4J_\Phi^2K_0\ln\frac{\Lambda}{\omega}+O(\omega)\ .\end{aligned}\tag{C.21}$$

## D: Non-Fermi liquid behavior

In this section, we provide details on calculating various physical observables, including the magnetic susceptibility, specific heat coefficient and the electrical conductivity. All of these calculations show non-Fermi liquid behavior.

### 1. Specific heat coefficient

We now outline the calculation of the anomalous exponent $\alpha$ in the specific heat coefficient

$$\gamma(T)=\frac{C_V}{T}\sim|g-g_c|^{-\alpha}\,\Gamma\left(\frac{T}{T_{FL}}\right)\tag{D.1}$$

in the strange metal state. One can refer to Ref. 10 for details.

The specific heat coefficient in the SM state is mainly contributed from the quadratic Gaussian fluctuation of the RVB field $\hat{\bar{\Phi}}_{\mathbf{k}}$ whose dynamics is described by the Hamiltonian $H_G$:

$$H_G=\sum_{\mathbf{k}}\hat{\bar{\Phi}}_{\mathbf{k}}(\varepsilon_\Phi(\mathbf{k})+m_\Phi)\hat{\bar{\Phi}}_{\mathbf{k}}.\tag{D.2}$$

To proceed, we evaluate the ensemble average of internal energy $\bar{E}_G$ for $\hat{\bar{\Phi}}_{\mathbf{k}}$, given by

$$\bar{E}_G=\sum_{\mathbf{k}}\frac{\varepsilon_\Phi(\mathbf{k})}{e^{\beta(\varepsilon_\Phi(\mathbf{k})+m_\Phi)}-1}=W_\Phi\int_{m_\Phi}^\Lambda d\varepsilon_\Phi\,\frac{\varepsilon_\Phi^{1+\epsilon/2}}{e^{\beta\varepsilon_\Phi}-1}.\tag{D.3}$$

Here, $V$ denotes the system volume, $\beta\equiv 1/T$, $\Lambda$ is the upper energy cutoff scale and

$$W_\Phi\equiv\frac{V\Omega_d}{2}\left(\frac{m^*\lambda^2\Lambda}{4\pi N_0J_\Phi^2J_\chi^2}\right)^{1+\epsilon/2}\tag{D.4}$$

denotes the density of states for the $\hat{\bar{\Phi}}_{\mathbf{k}}$ field with $\Omega_d\equiv 2\pi^{d/2}/\Gamma(d/2)$ being the solid angle of a $d$-dimensional sphere and $\Gamma(n)$ being the gamma function with argument $n$.

Taking into accounting for the renormalization of temperature $T(l)=Te^{zl}$ [17,18], the specific heat coefficient $\gamma(T)\equiv C_V/T$ is obtained by the definition $\gamma(T)\equiv T^{-1}\partial\bar{E}_G/\partial T$:

$$\begin{aligned}\frac{C_V}{T} &= e^{-\epsilon l}\,W_\Phi\int_{m_\Phi(l)}^\Lambda d\varepsilon_\Phi(l)\,\frac{\beta(l)^2\,\varepsilon_\Phi(l)^{2+\epsilon/2}\,e^{\beta(l)\varepsilon_\Phi(l)}}{\left(e^{\beta(l)\epsilon_\Phi(l)}-1\right)^2}\Bigg|_{l=l_0}\\ &= -\frac{1}{4}A(l_0)\left(\frac{T}{T_{FL}}\right)^{\epsilon/2}\int_{m_\Phi/T}^{m_\Phi\Lambda/T}dx\,\frac{x^{2+\epsilon/2}}{\sinh^2(x/2)}\end{aligned}\tag{D.5}$$

with $x\equiv\varepsilon_\Phi(l)/T(l)$ and the scale dependent prefactor $A(l_0)=e^{-\epsilon l_0}W_\Phi$. The second line in Eq. (D.5) is evaluated near the critical fixed point at which $m_\Phi(l)$ is renormalized to of order of one, $m_\Phi(l_0)\approx\mathcal{O}(1)\Rightarrow 1=m_\Phi e^{z\,l_0}=m_\Phi\xi^z$ with $m_\Phi$ being the bare mass of the $\hat{\bar{\Phi}}$-field, $\xi$ being the correlation length, and $T(l_0)=Te^{zl_0}\sim T\xi^z\sim T/T_{FL}$. In the above derivations, the relations $e^{l_0}=\xi$ and $\xi^z\sim T_{FL}^{-1}\sim(g-g_c)^{-1}\sim(J_\Phi-J_\Phi^*)^{-1}$ have been used since the RG flows along the direction of $J_\Phi$ with $J_\chi$ fixed at $J_\chi^*$ dominates the critical properties.

Following the scaling procedures in Ref. 10, we renormalize the specific heat coefficient via rescaling various quantities such as the Fermi wave vector $k_F$ and the conduction-electron density of states $N_0$ near the critical fixed point of the RG flow, giving rise to an additional rescaling factor in prefactor in Eq. (D.5):

$$A(l_0)\propto e^{-\epsilon l_0}W_\Phi\propto e^{-\epsilon\,l_0}\left(\frac{m^*\lambda^2\Lambda}{2N_0J_\Phi^2J_\chi^2}\right)^{1+\epsilon/2}.\tag{D.6}$$

The conduction-electron density of states is given by $N_0\sim m^*k_F^{d-2}$ and thus is scale invariant at two dimensional space. According to the scaling procedures in Section C, we should rescale the Fermi wavev vector $k_F$ as $k_F\to k_F/e^{l_0}$. The energy cutoff $\Lambda$ is invariant under rescaling. In addition, both the local $f$-electron operator and the Kondo fluctuation operator $\hat{\chi}$ acquire a change in their scaling dimension: $[f]\to[f]-\frac{\epsilon}{4}$ and $[\hat{\chi}]\to[\hat{\chi}]-\frac{\epsilon}{4}$ for the reason that the specific heat coefficient is analyzed around the critical fixed point where $J_\chi\to J_\chi\,e^{-\epsilon l_0/2}\equiv j_\chi(l_0)$. At the same time, due to the change in the bare scaling dimension of the $f$ operator, we have to rescale the Lagrange multiplier $\lambda$ as $\lambda\to\lambda\,e^{\epsilon l_0/2}$ (or equivalently $[\lambda]\to[\lambda]+\epsilon/2$) relative to fixed $j_\chi=j_\chi^*$. The change in the scaling dimension of $[f]$

and $[\hat{\chi}]$ generates a scaling phase prefactor $e^{2\epsilon l_0}$ in front of the dispersion of the $\hat{\hat{\Phi}}$ bosons, $\varepsilon_\Phi(\mathbf{k})$ (this phase factor $e^{2\epsilon l_0}$ comes from the leading non-vanishing self energy of $\hat{\hat{\Phi}}$ which contains three Green's functions of $f$ and one for $\hat{\chi}$), see Ref. 10.

Collecting all the contributions of $e^{l_0}$ and Using the relation $e^{l_0} \sim (g-g_c)^{-1/2}$ yields

$$\begin{aligned} A(l_0) &\propto e^{-\epsilon\, l_0} W_\Phi \\ &\propto (g-g_c)^{\epsilon/2} \cdot \left( \frac{(g-g_c)^{-\epsilon/2}}{(g-g_c)^{\epsilon/2}\cdot (g-g_c)^{\epsilon}} \right)^{1+\epsilon/2} \\ &= (g-g_c)^{-\alpha}, \end{aligned} \tag{D.7}$$

where $\alpha = 3\epsilon/2 + \epsilon^2$.

### 2. Dynamical magnetic susceptibility

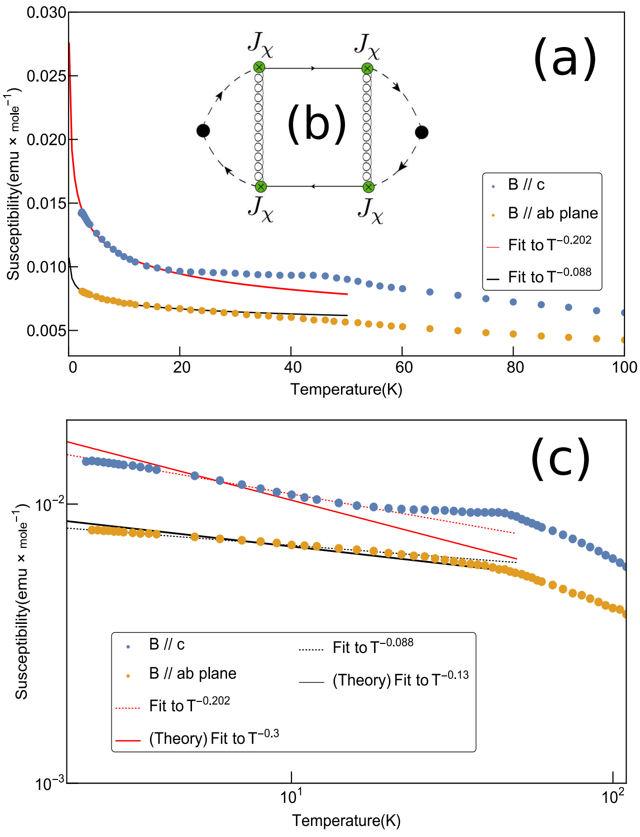


FIG. D.1: The magnetic susceptibility of $CeCoIn_5$ as a function of temperature: figure (a) and (c) show $\chi(T)$ in the linear and logarithmic scale, respectively. Inset (b) is the Feynman diagram to the $4^{\text{th}}$ order in $J_\chi$ for the local susceptibility $\chi_{\text{loc}}(T)$. In (b), each filled $\otimes$ symbol represents an interaction vertex of $J_\chi$.

At zero field and $T \ll T^*_{coh}$, we estimate the fractional exponent for the local spin susceptibility $\chi_{loc}(T)$ via power counting of the lowest non-trivial order diagram in Fig. D.1(b):

$$\chi_{loc}(T) \propto \frac{J_\chi^4}{T} \propto T^{2\epsilon-1} , \tag{D.8}$$

where the bare scaling for $[J_\chi] = \epsilon/2$ (or $J_\chi(T) \sim T^{-\epsilon/2}$) is used. Experimentally, the spin susceptibility along the $c$-axis shows a power-law behavior $\chi_{loc}(T) \sim T^{-p}$ with $p \approx 0.202$ [8]. When taking the optimized value of $\epsilon \sim 0.35$ fitted to the specific heat coefficient (the blue curve in Fig. 1(c) of the main text), we get $\chi_{loc}(T) \sim T^{2\epsilon-1} \sim T^{-\bar{p}}$ with $\bar{p} \approx 0.3$ (red solid line in Fig. D.1(c)), in reasonable agreement with the experiments (red dashed line in Fig. D.1(c)).

Due to magnetic anisotropy, magnetic susceptibility in the $ab$-axis and along the $c$-axis show different power-law singularity at low temperature. Theoretically, we obtain the power-law singularity in the spin susceptibility in the $ab$-plane $\chi_{loc}(T) \sim T^{-0.13}$ with an optimized extra dimension $\epsilon \sim 0.45$, as shown in the black solid line in Fig. D.1(c). It is not far away from the experimentally observed power-law behavior, $\chi_{loc}(T) \sim T^{-0.088}$ (black dashed line in Fig. D.1(c)) [8].

### 3. Electrical resistivity in the FL and the NFL regime

In this section, we compute the electrical resistivity in the FL ($T$-quadratic) and the $T$-linear regime, respectively. We further demonstrate that the resistivity is dominated by the NFL $T$-linear contribution in the NFL regime ($T \sim 10$K) via estimating the ratio between the $T$-quadratic and $T$-linear contributions.

The electrical conductance is, in general, contributed from the mobile $c$-electron and the local $f$-electron:

$$\sigma(T) = \sigma_0 + \sigma_c(T) + \sigma_f(T) \approx \sigma_0 + \sigma_c(T) , \tag{D.9}$$

where $\sigma_0$ is the residual resistivity at zero temperature, which cannot be determined from our approach, and $\sigma_c$ and $\sigma_f$ is the conductance contributed from the $c$- and $f$-electrons, respectively. In Eq. (D.9), we ignore $\sigma_f$ as we expect that the electrical conductance is likely to be dominated by the mobile $c$-electron. Experimentally, it is shown that $\sigma_0 \sim 0.5\,\mu\Omega^{-1}\cdot \text{cm}^{-1}$ [8].

Via the Boltzmann equation, the electrical resistivity can be computed through [19]

$$\sigma(T) = -\frac{2e^2}{3}\int \frac{dk^2}{(2\pi)^2} v_k^2 \tau(k) \frac{\partial n_F}{\partial \epsilon_k}, \tag{D.10}$$

where the group velocity is given by $v_k \equiv k/m$ with $m$ being the effective mass of the conduction electron, $n_F(x) = 1/(e^{x/k_B T}+1)$ being the Fermi-Dirac distribution and

$$\begin{aligned} \tau^{-1}(\omega) &= -2\sum_{\mathbf{k}} \text{Im}\Sigma_c(\omega^+,\mathbf{k}) , \\ \Sigma_c(\omega^+,\mathbf{k}) &= c_{imp}\, T_{\mathbf{kk}}(\omega^+) \end{aligned} \tag{D.11}$$

with $\Sigma_c$ being the self-energy, $\tau$ the life-time and $T_{\mathbf{kk}}$ being the $T$-matrix.

The conductance in the Fermi liquid regime follows a quadratic-in-$T$ behavior,

$$\begin{aligned}\sigma_{\rm FL}(T) &= a + \sigma_c(T)\\ &= a - \sigma_c^0\left(1 - \frac{\pi^2}{3}\left(\frac{k_BT}{a_c}\right)^2\right) \ , \end{aligned} \quad \text{(D.12)}$$

with $a$ being a temperature independent constant.

However, the authors of Ref. 10 found a linear-in-$T$ conductance in the non-Fermi liquid regime due to a linear-in-frequency behavior of the scattering rate:

$$\tau^{-1}(\omega) = -2{\rm Im}\ \Sigma_c(\omega) = -(\alpha - \gamma|\omega_\chi|) \quad \text{(D.13)}$$

with $\alpha = \pi J_\chi^2 N_0$ and $\gamma = 1/\pi$. In Eq. (D.13), the conduction-electron self energy $\Sigma_c$ is obtained from a second-order perturbation in $J_\chi$ (see Ref. 10 for details). From Eqs. (D.10) and (D.13), we have (see also Ref. 10)

$$\sigma_{\rm NFL}(T) = b - c(k_BT) \ . \quad \text{(D.14)}$$

In Eqs. (D.12) and (D.14), we define

$$\begin{aligned}\sigma_c^0 &= \frac{n_c e^2\hbar}{2m^* N_f|\chi|^2\Xi_c} \ , \ \frac{1}{a_c^2} = \frac{\sin^2 2\theta_c}{4\Xi_c\Delta_c\Lambda_f} \ ,\\ b &= \frac{e^2\epsilon_F\sqrt{2m\epsilon_F}}{24\pi^3\hbar^2 J_\chi^2 N_0} \ , \ c = \frac{\sqrt{2m\epsilon_F}\, e^2\epsilon_F}{24\pi^5\hbar^2 J_\chi^4 N_0^2} \ ,\end{aligned} \quad \text{(D.15)}$$

where $\Delta_c \equiv \pi|\chi|^2 N_0$, $\Xi_c \equiv \left|2\tan^{-1}\left(\frac{\Lambda_f}{\Delta_c}\right) - \pi\right|$ and $\theta_c \equiv \tan^{-1}(\Lambda_f/\Delta_c)$.

We choose the following input parameters in the following estimation: the effective mass of heavy electrons $m^* \sim 10^{-27}$ kg (about 1000 times heavier as much as the bare electrons), density of states of the $c$-electrons $N_0 \sim 10^2$ eV$^{-1}$, the bandwidth of the conduction electrons $\Lambda \sim 1$ eV, the band width for the $f$-electrons $\Lambda_f \sim 10^{-3}\Lambda \sim 10^{-3}$ eV, the density of states for the $f$-electrons $N_f \sim 1000 N_0 \sim 10^5$ eV$^{-1}$, the Fermi energy of conduction electron $\epsilon_F \sim 0.1$ eV and $J_\chi N_0 = \sqrt{\epsilon} \sim 0.5$, and the density of the conduction electrons is $n_c \sim 10^{22}$ cm$^{-3}$. The mean-field $\chi$ can be determined from Fig. A.1, $\chi \sim t \sim 1.5\times10^{-2}$ eV.

Resistivity is defined as the inverse of the conductivity, given by

$$\begin{aligned}\rho(T) &= \frac{1}{\sigma(T)}\\ &= \frac{1}{\sigma_0}\left[1 + \frac{c}{\sigma_0}(k_BT) + \frac{\sigma_c^0}{\sigma_0}\left(\frac{k_BT}{a_c}\right)^2\right] \ .\end{aligned} \quad \text{(D.16)}$$

At $T$ =10K (in the non-Fermi liquid regime), the ratio of the resistivity (only the temperature dependent terms) in the Fermi liquid and the non-Fermi liquid regime is estimated as

$$\frac{\frac{\sigma_c^0}{\sigma_0^2}\left(\frac{k_BT}{a_c}\right)^2}{\frac{c}{\sigma_0^2}(k_BT)} = \frac{\sigma_c^0}{c}\left(\frac{k_BT}{a_c}\right) \sim 10^{-16} \ . \quad \text{(D.17)}$$

We thus demonstrate that the electrical resistivity at the NFL regime is dominated by NFL linear-in-$T$ contribution.

* Electronic address: cdshjtr.ep02g@nctu.edu.tw
† Electronic address: chung@mail.nctu.edu.tw

[1] J. S. Van Dyke, F. Massee, M. P. Allan, J. C. S. Davis, C. Petrovic, D. K. Morr, PNAS **111**, 11663-11667 (2014).
[2] S. Zaum, K. Grube, R. Schäfer, E. Bauer, J. D. Thompson, H. V. Löhneysen, Phys. Rev. Lett. **106**, 087003 (2011) .
[3] O. Erten, R. Flint, and P. Coleman, Phys. Rev. Lett. **114**, 027002 (2015).
[4] C. H. Booth, T. Durakiewicz, C. Capan, D. Hurt, A. D. Bianchi, J. J. Joyce, and Z. Fisk, Phys. Rev. B **83**, 235117 (2011).
[5] See, for example, M. Tinkham, in *Introduction to superconductivity* (Dover Publications, New York, 2004).
[6] Q. Y. Chen *et at.*, J. Phys Condens. Matter **96**, 045107 (2017).
[7] J. Paglione,T. A. Sayles, P.-C. Ho, J. R. Jeffries, and M. B. Maple, Nature **3**, 703-706 (2007).
[8] C. Petrovic, P. G. Pagliuso, M. F. Hundley, R. Movshovich, J. L. Sarrao, J. D. Thompson, Z. Fisk, and P. Monthoux, J. Phys. Condens. Matt. **13**, L337-L342 (2001).
[9] S. Burdin, A. Georges, and D. R. Grempel, Phys. Rev. Lett. **85**, 1048-1051 (2000).
[10] Y. Y. Chang, S. Paschen, and C. H. Chung, Phys. Rev. B **97**, 035156 (2018).
[11] J. Ye and S. Sachdev, Phys. Rev. B **44**, 10173 (1991).
[12] S. J. Yamamoto and Q. Si, Phys. Rev. B **81**, 205106 (2010).
[13] Q. Si, S. Rabello, K. Ingersent, and J. L. Smith, Phys. Rev. B **68**, 115103 (2003).
[14] L. Zhu and Q. Si, Phys. Rev. B **65**, 024426 (2002).
[15] M. Nicklas, O. Stockert, Tuson Park, K. Habicht, K. Kiefer, L. D. Pham, J. D. Thompson, Z. Fisk, and F. Steglich, Phys. Rev. B **76**, 052401 (2007).
[16] For a 0.05% doping of Cd [15], we expect the average unpaired electrons of the Ce atom will increase by 0.15 as some of the In atoms with $In^{1+}$ oxidation state in the $CeIn_3$ layer are replaced with Cd atoms ($Cd^{2+}$). The valence fluctuation (0.8 ∼ 0.9) leads to a nearly half-filled of the $f$-electron. The average occupation number per site turns out to be $n_f = (1+0.15)\times0.8 = 0.92$ to $n_f = (1+0.15)\times0.9 = 1.03$. Hence, it is reasonable to approximate the Lagrange multiplier $\lambda \to \infty$ in our RG calculation.
[17] A. J. Millis, Phys. Rev. B **48**, 7183 (1993).
[18] J. Hertz, Phys. Rev. B **14**, 1165-1184 (1976).

[19] A. C. Hewson, in *The Kondo problem to heavy fermions*, Vol. 2. (Cambridge university press, Cambridge, England, 1997).

[20] Q. Y. Chen *et al.*, Phys. Rev. Lett. **120**, 066403 (2018) .
